# Supplementary material for: DiffGraph: Heterogeneous Graph Diffusion Model
Source: arXiv:2501.02313 source file (2025-01-04)
Supplement: Supplementary file 1 [file appendix.tex]

\section{Appendix}
